# Supplementary material for: Systematic construction of continuous-time neural networks for linear dynamical systems
Source: arXiv:2403.16215 source file (2024-03-24)
Supplement: Supplementary file 1 [file supplemental_material.tex]

\section{Supplemental material}

\subsection{Some details on clustering algorithm}
\label{ss:sm_clustering}
The parameter \texttt{Clustering algorithm} in Algorithm \ref{alg:preprocessing_lti} can be chosen as any of the vast variety of clustering algorithms to  cluster eigenvalues of the state matrix $A$.
These include the well-known k-means algorithm \cite{lloyd1982least}, the spectral clustering algorithm \cite{von2007tutorial}, and others.
% First, we cluster the eigenvalues using well-known clustering algorithms, for instance, k-means, affinity propagation, spectral clustering, Ward hierarchical clustering, and Agglomerative clustering. 
These algorithms and many more are implemented in the Python package scikit learn \cite{scikit-learn}. 
For each cluster of eigenvalues, we identify the eigenvalue with the largest real part and sort the clusters in descending order based on these. This step is not necessary, but it ensures that the algorithm is deterministic. Within each cluster of eigenvalues, we order the eigenvalues according to the absolute value of the real part in ascending order. This is required to ensure that for a cluster having real and complex eigenvalues, the real eigenvalues are placed first. This ensures a suitable sparsity pattern of the diagonal block (as shown in the matrix on the right in equation \eqref{eq:sparsity_patterns}), which is exploited in Theorem \ref{th:parameter_maps}. 

\subsection{Additional numerical examples}
\subsubsection{A toy example with all kinds of eigenvalue clusters}
The nature of eigenvalues of each block of the state matrix, i.e., whether they are real or complex, decides whether neurons in the corresponding HHL are first-order or second-order (See Definition \ref{def_io_neuron}). 
Each HHL can thus be categorized into three types, such that the HHL consists of either only first-order neurons, or only second-order neurons, or both. 
The goal of the following toy example is to demonstrate that a dynamic neural network consisting of all kinds of the abovementioned HHLs can simulate an LTI system accurately and thus validate the implementation.

We construct an LTI system with input, state, and output dimensions $d_i = 10$, $d_h = 19$ and $d_o = 4$. The state matrix $A \in \mathbb{R}^{19 \times 19}$ is block upper triangular, with all entries above the diagonal blocks equal to $-0.5$ (an arbitrary choice). 
Figure \ref{fig:eg_all_clusters_1} shows the eigenvalues of the state matrix. 
There are six pairs of complex eigenvalues $\lambda_j = a_j \pm i b_j$ for $j \in {1, 2, \hdots, 6}$ which lie on the first six $2 \times 2$ diagonal blocks of the state matrix as $\begin{bmatrix}
    a_j & -b_j \\
    b_j & a_j
\end{bmatrix}$ and the seven real eigenvalues lie on the last seven diagonal blocks of the state matrix as $1 \times 1$ blocks in any order.  
We choose the elements of the input matrix $B \in \mathbb{R}^{19 \times 10}$ and the output matrix $C \in \mathbb{R}^{4 \times 19}$ randomly from a uniform distribution over $[0, 1)$. The elements of feedforward matrix $D \in \mathbb{R}^{4 \times 10}$ are chosen randomly from a uniform distribution over $(-1, 0]$. 

Figure \ref{fig:eg_all_clusters_1} shows how the eigenvalues are clustered with different colors indicating different clusters. 
Figure \ref{fig:eg_all_clusters_2} shows the corresponding hidden layer architecture of the constructed DyNN with depth (number of neurons in a given HHL) of each HHL corresponding to the respective eigenvalue cluster. 
\newline
\begin{minipage}{0.35\textwidth}
    \centering    
\includegraphics[height=0.9\textwidth,width=\textwidth]{figures/fig3_1.pdf}
    \captionof{figure}{Eigenvalue clusters}
    \label{fig:eg_all_clusters_1}
\end{minipage}\hspace{0.5cm}
\begin{minipage}{0.35\textwidth}
    \includegraphics[height=0.9\textwidth, width=\textwidth]{figures/fig3_2.pdf}
    \captionof{figure}{DyNN architecture: hidden layers}
    \label{fig:eg_all_clusters_2}
\end{minipage}\hspace{0.5cm}

Figure \ref{fig:eg_all_clusters_3} compares the output of the numerical solution using a Scipy routine signal.lsim with the output of the dynamic neural network. Finally, Figure \ref{fig:eg_all_clusters_4} shows that the relative and absolute errors between the outputs of the numerical solver and dynamic neural network are extremely small, thereby validating the implementation.
\begin{center}
    \includegraphics[width=0.9\textwidth]{figures/mixed_evals_sol.pdf}   
    \captionof{figure}{Comparison of outputs of the dynamic neural network and the numerical solver.}
    \label{fig:eg_all_clusters_3}

    \includegraphics[width=0.9\textwidth]{figures/mixed_evals_err.pdf}   
    \captionof{figure}{Error between the outputs of the dynamic neural network and the numerical solver.}
    \label{fig:eg_all_clusters_4}
    
\end{center}

%%%%%% New plots %%%%%%%%%%%%%%%%%%
\subsubsection{Convection-Diffusion equation: State matrix with closely clustered eigenvalues}
\label{app:ss:convection}
A two-dimensional transient convection-diffusion equation is
% Equation
\begin{align} \label{eq:conv_diff}
    \frac{\partial T}{\partial t} = \mathcal{D} \Bigl(\frac{\partial^2 T}{\partial x^2} + \frac{\partial^2 T}{\partial y^2}\Bigr) - v_x \frac{\partial T}{\partial x} - v_y \frac{\partial T}{\partial y} + \mathcal{S}, 
\end{align}
where T is the variable of interest (concentration of species or temperature), $\mathcal{D}$ is diffusivity, $v_x$ and $v_y$ are drift velocities in x and y directions, and $S$ is the source term. 
We interpret this as a system with $S$ as the input and the solution $T$ as the output.
% Parameters
The spatial domain is $[0, 10] \times [0, 9.5]$ with 20 grid points in each dimension. 
The right and left boundaries are periodic. The boundary conditions at the top and bottom boundaries are Dirichlet with $T(x, 0) = T(x, 9.5) = 0$. 

The initial condition $T(x,y,0) = 0$. 
The velocities in x and y dimensions are given by $v_x= 0.6$ and $v_y = 0$, and the diffusivity $\mathcal{D} = 1.4$. 
Let $t_d$ be a uniform grid in $[0,10]$ in steps of $0.1$.
Heat is injected into the system via the source term at time $t = 0.2$ as a Gaussian:
\iffalse
    $\mathcal{S}(x, y, t)=100 \exp{\Bigl( -0.8\bigl((x-l/2)^2 +(y-l/2)^2)\bigr)\Bigr)}\delta(t-0.2)$ where $\delta$ is the dirac-impulse.
\fi
\textcolor{red}{
\begin{equation*}
\mathcal{S}(x, y, t) = \begin{cases}
     100 \exp{\Bigl( -0.8\bigl((x-l/2)^2 +(y-l/2)^2)\bigr)\Bigr)} \quad \textnormal{if } t=0.2,\\
     0 \quad \quad \textnormal{otherwise},
 \end{cases}    
 \end{equation*}
}
and is interpolated piecewise linearly for the time points in between.
\iffalse
We inject heat into the system via the source term at time $t = 0.2$ as a Gaussian impulse: 
$\mathcal{S}(x, y, t) = 100 \exp{\Bigl( -0.8\bigl((x-l/2)^2 +(y-l/2)^2)\bigr)\Bigr)}\delta(t-0.2)$ where $\delta$ is the dirac-impulse.
\fi

% Problem setting
We choose a uniform grid in space, and the gradient and Laplacian operators are discretized with second-order finite differences at each grid point $(i, j)$ as $\frac{\partial T}{\partial x}\big|_{i,j} \approx \frac{T_{i+1,j} - T_{i-1,j}}{2h}$, $\frac{\partial T}{\partial y}\big|_{i,j} \approx \frac{T_{i,j+1} - T_{i,j-1}}{2h}$ and $(\frac{\partial^2 T}{\partial x^2} + \frac{\partial^2 T}{\partial y^2})\big|_{i,j} \approx \frac{T_{i+1, j} + T_{i-1, j} + T_{i, j+1} + T_{i, j-1} - 4T_{i, j}}{h^2}$. 
The spatially discretized form of equation \eqref{eq:conv_diff} is an LTI system, where the state variable is represented by $T$. The spatial discretization scheme dictates the sparsity pattern and the elements of the state matrix $A \in \mathbb{R}^{400 \times 400}$. The other state-space matrices are $B = \mathcal{I}_{400}$, $C = \mathcal{I}_{400}$ and $D = 0$. 

\begin{figure}
\begin{center}
\includegraphics[width=0.9\textwidth]{figures/conv_diff_sep_0.pdf}
    \captionof{figure}{Eigenvalue clusters of the state matrix (color bar indicates eigenvalue clusters)}
    \label{fig:eigenvalue_clustering}
\end{center}
\end{figure}

\begin{figure}
    \begin{center}
        \begin{minipage}{0.3\textwidth}
        \includegraphics[height=0.9\textwidth, width=\textwidth]{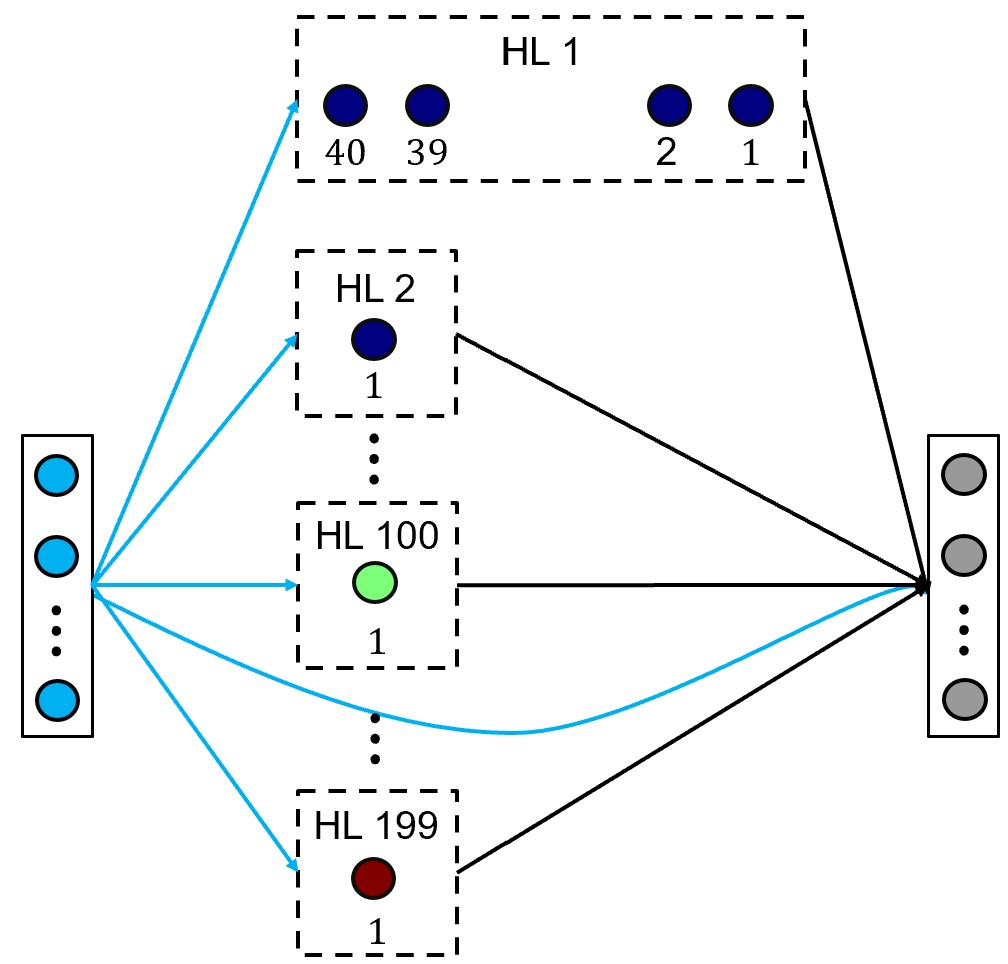}
        \captionof{figure}{DyNN architecture (color bar indicates HHLs)}
        \label{fig:DyNN_architecture}
        \end{minipage}\hspace{0.2cm}
        %%%%%% New plots %%%%%%%%%%%%%%%%%%
        \begin{minipage}{0.3\textwidth}
            \includegraphics[height=0.9\textwidth,width=\textwidth]{figures/n_conv_diff_sep_3.pdf}
            \captionof{figure}{Number of function (right-hand side of the ODE) evaluations required by the ODE solver in each neuron averaged over HHLs (color bar indicates HHLs)}
            \label{fig:cd_nfe}
        \end{minipage}
    \end{center}
\end{figure}
\begin{figure}
    \begin{center}
    \includegraphics[width=0.95\textwidth]{figures/n_conv_def_2_comparison.pdf}   
    \captionof{figure}{Convection-diffusion equation: dynamic neural network solution (top panel), numerical solution using a python routine scipy.signal.lsim (middle panel), the absolute error between the two solutions (bottom panel) at five time instances shown at the top.}
    \label{fig:n_timesteps_comparison}
\end{center}
\end{figure}
We simulate the semi-discretized LTI system with a DyNN and compare the results with ones obtained from the classical numerical solver that simulates the LTI system using the Python routine Scipy.signal.lsim.
After preprocessing the LTI system with Algorithm \ref{alg:preprocessing_lti}, the state matrix is block-diagonalized. 

Figure \ref{fig:eigenvalue_clustering} shows how the eigenvalues are clustered. The state matrix in this case is not normal and hence not unitarily diagonalizable. 
Moreover, the state matrix has a repeated eigenvalue - $0$ with an algebraic multiplicity of 40. 
% Since the states corresponding to the top and bottom boundaries are fixed, the rows of the state matrix corresponding to these states are all zero, leading to zero eigenvalues with a multiplicity of 40.
Thus, these must be clustered together, resulting in one horizontal layer with 40 neurons. Figure \ref{fig:DyNN_architecture} shows the resulting architecture, where the first HHL has 40 neurons and the rest have 1 neuron each. The condition number of the transformation matrix in this case is $C_{tr} = 7.42$. If the number of clusters is increased by $1$, the repeated eigenvalues are forced to be in different clusters, which is not possible and the clustering algorithm fails. 

Figure \ref{fig:cd_nfe} shows the Number of Function Evaluations (NFE) in the ODE solver averaged over the neurons of each horizontal layer. As the state dynamics are decoupled across the horizontal layers, the horizontal layers that require a lower NFE to solve the ODE to a prescribed tolerance are not forced to use a higher NFE as required by the other horizontal layers.  
Finally, Figure \ref{fig:n_timesteps_comparison} demonstrates that the DyNN simulates the semi-discretized convection-diffusion system accurately up to machine precision compared to the numerical solver.
%%%%%% New plots %%%%%%%%%%%%%%%%%%

%%%%%% New plots %%%%%%%%%%%%%%%%%%
\begin{remark}
The right boundaries are not included as state variables in the finite difference discretization, as they are the same as the left boundary points. However, the top and bottom boundaries which are fixed, are included as the state variables, where the gradient with respect to time does not change. For convenience, the domain sizes are adapted to keep the discretization width $h_x = h_y = 0.5$.   
\end{remark}

\section{Extra figures of the examples in the main paper}
\label{app:sss:extra_figures}
\subsection{Diffusion Equation (Example 1 from the main text)}
\begin{center}
\includegraphics[width=0.9\textwidth]{figures/diffusion_solution_err.pdf}   
    \captionof{figure}{Diffusion equation: dynamic neural network solution (top panel), numerical solution using a python routine scipy.signal.lsim (middle panel), the absolute error between the two solutions (bottom panel) at five time instants.}
    \label{fig:diffusion_solution}
\end{center}
\iffalse
\begin{figure}
    \centering
    \begin{minipage}{0.3\textwidth}
    \includegraphics[height=0.9\textwidth,width=\textwidth]{figures/diff_sep_3.pdf}
    \captionof{figure}{Number of evaluations of the right-hand side of the ODE corresponding to each neuron (color bar indicates different neurons/HHLs)}
    \label{fig:diff_nfe}
\end{minipage}
\end{figure}
\fi

\subsection{State matrix with different kinds of clusters of eigenvalues (Example 3 from the main text))}
\begin{center}
    \begin{minipage}{0.32\textwidth}
    \includegraphics[height=0.9\textwidth,width=\textwidth]{figures/mixed_evals_3.pdf}
    \captionof{figure}{Number of function (right-hand side of the ODE) evaluations required by the ODE solver in each neuron averaged over HHLs (color bar indicates HHLs)}
    \label{fig:nfe_blobs}
\end{minipage} \hspace{0.3cm}
\begin{minipage}{0.3\textwidth}
    \includegraphics[height=0.9\textwidth,width=\textwidth]{figures/conv_diff_sep_3.pdf}
    \captionof{figure}{Number of function (right-hand side of the ODE) evaluations required by the ODE solver in each neuron averaged over HHLs (color bar indicates HHLs)}
    \label{fig:nfe}
\end{minipage}\hspace{0.2cm}
\end{center}
\begin{center}
    \includegraphics[width=0.99\textwidth]{figures/mixed_evals_sol.pdf}   
    \captionof{figure}{Comparison of outputs of the dynamic neural network and the numerical solver.}
    \label{fig:sol_blobs}
    % Error
    \includegraphics[width=0.99\textwidth]{figures/mixed_evals_err.pdf}   
    \captionof{figure}{Error between the outputs of the dynamic neural network and the numerical solver.}
    \label{fig:error_blobs}
\end{center}

\subsection{Convection-Diffusion equation (Example \ref{app:ss:convection} from supplemental text)}
\begin{center}
    \includegraphics[width=0.95\textwidth]{figures/conv_def_2_comparison.pdf}   
    \captionof{figure}{Convection-diffusion equation: dynamic neural network solution (top panel), numerical solution using a python routine scipy.signal.lsim (middle panel), the absolute error between the two solutions (bottom panel) at five time instances shown at the top.}
    \label{fig:timesteps_comparison}
\end{center}
